# Supplementary material for: Using eye tracking to investigate what native Chinese speakers notice about linguistic landscape images
Source: arXiv:2312.08906 source file (2024-07-02)
Supplement: Supplementary file 1 [file appendices.tex]

\section{TTT, by Piet Hein}
Problems worthy \\
of attack \\
prove their worth \\
by hitting back. \\
\\
Put up in a place \\
where it's easy to see \\
the cryptic admonishment\\
    T.T.T. \\
\\
When you feel how depressingly \\
slowly you climb, \\
it's well to remember that\\
Things Take Time. \\
\\
The road to wisdom? - Well, it's plain\\
and simple to express: \\
   Err \\
   and err \\
   and err again \\ 
   but less \\
   and less \\
   and less. \\

\begin{center}
    \includegraphics[width=\linewidth,height=7cm]{src/figures/brighton.jpeg}
    \captionof{figure}{This is a figure in the appendix}
\end{center}
