# Supplementary material for: Using eye tracking to investigate what native Chinese speakers notice about linguistic landscape images
Source: arXiv:2312.08906 source file (2024-07-02)
Supplement: Supplementary file 2 [file resources.tex]

\section{Key resources}
Here could be a nice table of your resources. 

% Make your own table style https://tex.stackexchange.com/questions/94799/how-do-i-color-table-columns
